# Supplementary material for: Closing the Gap: Joint De-Identification and Concept Extraction in the Clinical Domain
Source: arXiv:2005.09397 source file (2020-05-19)
Supplement: Supplementary file 1 [file supplementary.tex]

\appendix

\reviewerTodo{R1}{Supplementary material: I miss more details about the implementation of the methods, i.e., which programming language, libraries or frameworks have been used. (may include this on the additional page)}

\newContent{
We use PyTorch for all models and the FLAIR library~\cite{emb/akbik2018}. Our published code will include classes compatible with FLAIR version 0.4.5 that can be used directly within the existing framework and classes. 
}
	
\section{Data Preprocessing}
We used the propressing scripts from ~\newcite{i2b2/alsentzer2019} for the English i2b2 corpora and the Spanish Clinical Case Corpus tokenizer~\cite{spaccc/Intxaurrondo19} for both Spanish corpora. We noticed that the Spanish tokenizer sometimes merges multi-word expressions into a single token joined with underscores for contiguous words. As a result, some tokens cannot	be aligned with the corresponding entity annotations. To address this, we split those tokens into their components in a postprocessing step.
	
\section{Hperparameters}
The embeddings have 300 (byte-pair-encoding), 300 (fastText), 100 (domain-specific fastText),
and 4,048 (FLAIR) dimensions. The clinical BERT embeddings have 768 dimensions and are constructed by averaging the last four layers with the scalar mix operation proposed by~\cite{liu-etal-2019-linguistic}. 
As described in Section 3, we concatenate them to one input vector, resulting in a total input dimensionality of 5,416 for English and 4,748 for Spanish. For the LSTM, we use 256 hidden units per direction.
The task-specific hidden layer of the multitask model has 128 units.
Note that we use the same hyperparameters for all our models and all tasks.
	
\section{Training}
For training, we use stochastic gradient descent with a learning rate of 0.1 and a batch size of 32 sentences. The learning rate is halved after 3 consecutive epochs without improvement on the development set.
For the joint models, we pre-train the anonymization part for 3 epochs and, then, use a higher initial learning rate of 0.2 for the concept extraction part. 
We perform early stopping on the hold-out development set, or create a new development set with 10\% of the training set size whenever no development set was provided (i2b2 2010 corpus) or the original training and development set were combined.
